# Supplementary material for: Privacy-Engineered Value Decomposition Networks for Cooperative Multi-Agent Reinforcement Learning
Source: arXiv:2311.06255 source file (2023-09-13)
Supplement: Supplementary file 1 [file appendix.tex]

\section*{Appendix}
\subsection{Proof of Theorem 1}
By the end of the training, let $D$ denote the set of all episodes that have been loaded onto an agent's replay buffer in sequential order. That is $d_1 \in D$, is the first episode, $d_2$ is the second episode, and so forth. Define
\begin{align}
    &D_1 = \{d_1\} \nonumber\\
    &D_2 = \{d_1, d_2\} \nonumber\\
    &\vdots\nonumber\\
    &D_{\texttt{buffer\_size}} = \{d_1,d_2,\dots, d_{\texttt{buffer\_size}}\}\nonumber\\
    &D_{{\texttt{buffer\_size}}+1}=\{d_2, d_3,\dots, d_{\texttt{buffer\_size}+1}\}\nonumber\nonumber\\
    \vdots \nonumber
\end{align}
At every iteration $i$ of Algorithm \ref{alg: contribution}, the algorithm applies the DP-SGD algorithm to $D\cap D_i$. With fixed sampling rate $p$, noise variance $\sigma^2$, and $\delta$, for all $i\in\mathbb{N}$, let $(\epsilon_i, \delta)$ be the differential privacy level of a single epoch of DP-SGD with $n=i$. By differential privacy's basic sequential composition theorem \cite{}, $k$ iterations of Algorithm \ref{alg: contribution} achieves $\left(\sum_{i=1}^k \epsilon_i, k \cdot \delta\right)$-differential privacy. However, this differential privacy level is tight and often overly conservative. More sophisticated composition theorems such as the Advanced Composition Theorem \cite{} or the Moments Accountant method for the case of DP-SGD can improve the bound. 

Notice that every episode is only used in Algorithm \ref{alg: contribution} for $t=\texttt{buffer\_size}$ iterations, and once the episode is replaced in the replay buffer with a new one, it is no longer a part of the training. The composition theorem in \cite{} can leverage such special set overlaps to provide better differential privacy bounds. In particular, let
\begin{equation}
    I = \left\{ \Tilde{D} \subseteq D \mid \bigcap_{d\in \Tilde{D}} d \neq \varnothing\right\}.
\end{equation}
Then, the differential privacy level of Algorithm \ref{alg: contribution} is upper bounded by the maximal differential privacy level of the composition of the DP-SGD algorithm using the sets in $I$. By fixing $p$, $\sigma$, and $\delta$, each application of the DP-SGD algorithm in the composition enforces the same level of differential privacy. As a result, the differential privacy level of Algorithm \ref{alg: contribution} corresponds to at most $\texttt{buffer\_size}$ compositions. Therefore, using the Moments Accountant for $\texttt{replay\_buffer}$ epochs computes the differential privacy level of Algorithm \ref{alg: contribution}.

Finally, the \texttt{buffer\_throughput} hyperparameter allows for Algorithm \ref{alg: contribution} to boost the differential privacy by the Subsampling Theorem \cite{abadi2016deep}. In particular, a $\texttt{buffer\_throughput}\ge 1$ enhances both $\epsilon$ and $\delta$ by a factor of $\texttt{buffer\_throughput}^{-1}$.
